# Supplementary material for: SuRe: Summarizing Retrievals using Answer Candidates for Open-domain QA of LLMs
Source: arXiv:2404.13081 source file (2024-04-17)
Supplement: Supplementary file 1 [file supp_rank_examples2.tex]

\begin{figure*}[t]
\vspace{-0.1in}
\begin{center}
    \includegraphics[width=0.8\textwidth]{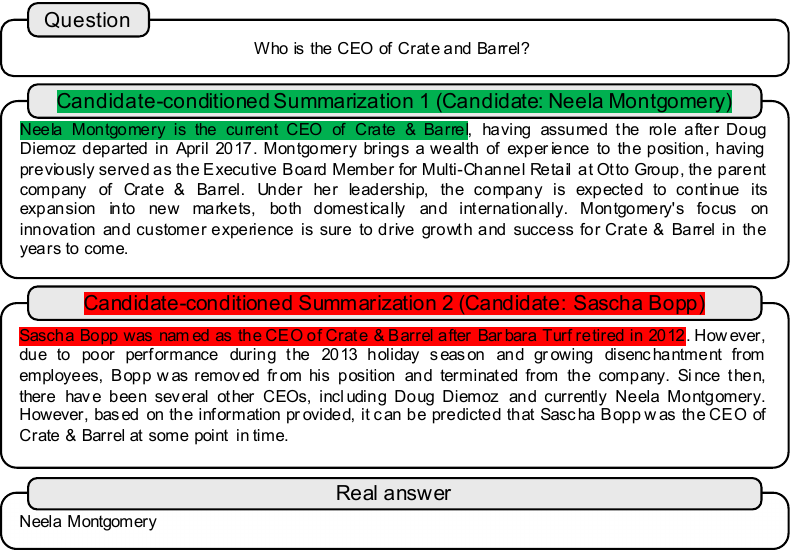}
\end{center}
\vspace{0.2in}
\begin{center}
    \includegraphics[width=0.8\textwidth]{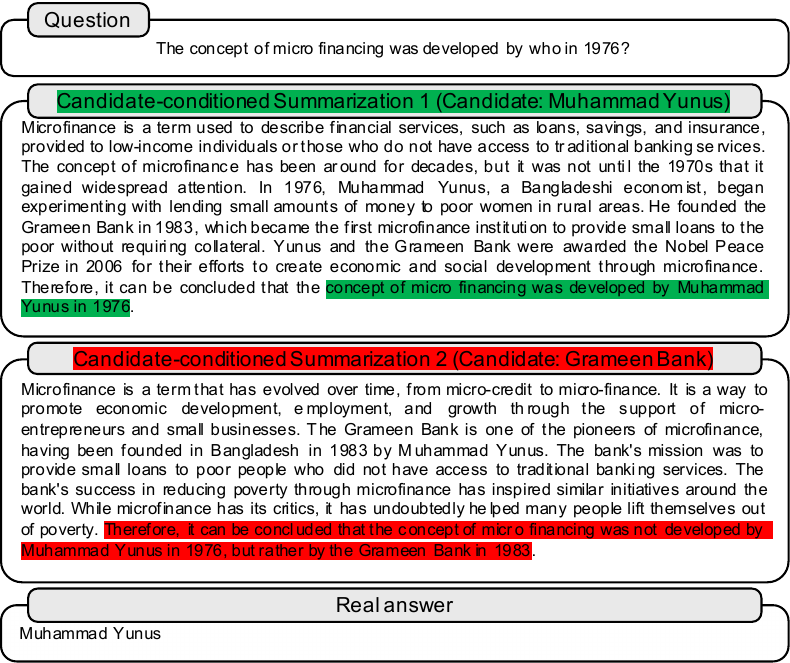}
\end{center}
\vspace{0.2in}
\begin{center}
    \includegraphics[width=0.8\textwidth]{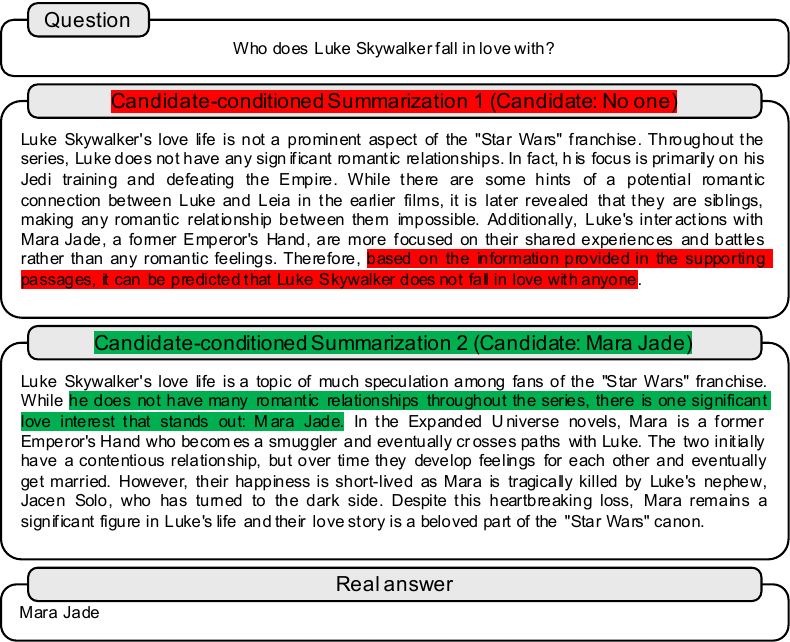}
\end{center}
\vspace{-0.1in}
\caption{Examples of }
\vspace{-0.1in}
\label{fig:supp_rank}
\end{figure*}
